# Supplementary material for: Identification of Spikes in Time Series
Source: arXiv:1801.08061 source file (2018-01-24)
Supplement: Supplementary file 1 [file Supplemental_Material.tex]

rm(list = ls())
ls() 

library(tsoutliers) 
library(forecast)
library(KFAS)
library(wavethresh)
library(EbayesThresh)
library(TSA)
library(ggplot2)
library(RColorBrewer)
library(grid)

##########################################################################
            # Define functions for spike detection methods #
##########################################################################

####### ARIMA ####### 

ar.out <- function(ts,shocks) {
	
	arfit <- auto.arima(ts,allowdrift=T,allowmean=T) 
	resid <- residuals(arfit)

# locate shocks identified by procedure 
	idsh <- time(resid)[resid>2*sd(resid)]

# calculate relative frequency of correctly identifying outliers 
	rfreq <- mean(as.numeric(shocks %in% idsh))

# calculate average frequency of misidentifying outliers 
	afreq <- sum(as.numeric(!idsh %in% shocks))

	freq <- rbind(rfreq, afreq)
	#print("arima")
	#print(freq)
	return(freq)
	}
	
####### Kalman ####### 

kfs.out <- 	function(ts,shocks) {
	
    fit <- auto.arima(ts,allowdrift=T,allowmean=T) 	
	coef <- 	fit$coef

# get coefficients and order of differencing
	try(rm(ar))
		if (is.na(coef["ar1"])) ar <- NULL
		if (!is.na(coef["ar1"])) ar <- coef["ar1"]
		if (!is.na(coef["ar2"])) ar <- c(ar,coef["ar2"])
		if (!is.na(coef["ar3"])) ar <- c(ar,coef["ar3"])
		if (!is.na(coef["ar4"])) ar <- c(ar,coef["ar4"])
		if (!is.na(coef["ar5"])) ar <- c(ar,coef["ar5"])

try(rm(ma))
		if (is.na(coef["ma1"])) ma <- NULL
		if (!is.na(coef["ma1"])) ma <- coef["ma1"]
		if (!is.na(coef["ma2"])) ma <- c(ma,coef["ma2"])
		if (!is.na(coef["ma3"])) ma <- c(ma,coef["ma3"])
		if (!is.na(coef["ma4"])) ma <- c(ma,coef["ma4"])
		if (!is.na(coef["ma5"])) ma <- c(ma,coef["ma5"])

diff <- fit$arma[length(fit$arma)-1]

# fit Kalman filter and smoother
	model <- SSModel(ts ~ SSMarima(ar=ar,ma=ma,d=diff))
	fit <- fitSSM(model,inits=c(0,0))
	out.kfs <- KFS(fit$model)

# calculate residuals
resid <- ts - out.kfs$muhat 

# locate shocks identified by procedure 
	idsh <- time(resid)[resid>2*sd(resid)]

# calculate relative frequency of correctly identifying outliers 
	rfreq <- mean(as.numeric(shocks %in% idsh))

# calculate average frequency of misidentifying outliers 
	afreq <- sum(as.numeric(!idsh %in% shocks))

	freq <- rbind(rfreq, afreq)
	#print("kalman")
	#freq
	return(freq)
	
	}
	
####### Wavelets ####### 

s.wave.out <- function(ts,shocks) {

# apply wavelet transform and get coeffcients
	ws <- append(ts[1:96],rep(0,32))
	wmap <- wd(ws)
	smap <- threshold(wmap,type="soft",policy="universal")

	sfit <- wr(smap)
	
# calculate residuals	
	resid <- ws[1:96] - sfit[1:96]
		
# locate shocks identified by procedure 
try(rm(idsh))
	idsh <- time(resid)[resid>2*sd(resid)]

# calculate relative frequency of correctly identifying outliers 
try(rm(rfreq))
	rfreq <- mean(as.numeric(shocks %in% idsh))
	#print(rfreq)

# calculate average frequency of misidentifying outliers 
try(rm(afreq))
	afreq <- sum(as.numeric(!idsh %in% shocks))
	#print(afreq)

	freq <- rbind(rfreq, afreq)
	#print("wavelet, soft thresholding")
	#print(freq)
	return(freq)

}	

####### Outlier Detection ####### 

d.out <- function(ts,shocks) {
	
	arfit <- auto.arima(ts,allowdrift=T,allowmean=T) 
	dAO <- detectAO(arfit)

# locate shocks identified by procedure 
	idsh <- unique(dAO$ind[dAO$lambda2>0])

# calculate relative frequency of correctly identifying outliers 
	rfreq <- mean(as.numeric(shocks %in% idsh))

# calculate average frequency of misidentifying outliers 
	afreq <- sum(as.numeric(!idsh %in% shocks))

	freq <- rbind(rfreq, afreq)
	#print("arima")
	#print(freq)
	return(freq)
	}

##########################################################################
                 # Define initial ARIMA models #
##########################################################################
set.seed(42654)

setwd("filepath")
source('./scripts/arima.R')
source("./scripts/tsoutliers.R")
source("./scripts/kfs.R")
source("./scripts/tsay.R")
source("./scripts/swavelet.R")
source("./scripts/hwavelet.R")
source("./scripts/ebt_wavelet.R")
source("./scripts/detectO.R")

# define iteration parameters
shock.num <- 1:10
shock.mag <- seq(0.1,0.5, by=0.1)

# Oakland parameters
oak.sim <-  function(iteration) arima.sim(n=96,list(order = c(4,1,2), ar = c(0.8481,-0.1436,0.3572,-0.6178), ma=c(-1.6616,0.7814)) , sd = c(0.0926, 0.1150,0.1129,0.0841,0.0812,0.0773,11.79155)) + 79.27858

# Richmond parameters
rich.sim <- function(iteration) arima.sim(n=96,list(order=c(0,1,1), ar = NULL, ma = c(-0.7940)),sd=c(0.0665, 12.49071)) + 73.68784

# Los Angeles parameters
la.sim <-  function(iteration) arima.sim(n=96,list(order=c(1,0,0),ar=c(0.436),ma=NULL), sd=c(0.093, 3.401935)) + 35.52811 

# Fresno parameters 
fres.sim <- function(iteration) arima.sim(n=96, list(order=c(1,1,1), ar=c(0.5306), ma=c(-0.9504)), sd=c(0.0966, 0.0319, 6.384975)) + 49.20486

# Sacramento parameters 
sac.sim <- function(iteration) arima.sim(n=96, list(order=c(2,0,1), ar=c(-0.465,0.5180), ma=c(0.9315)), sd=c(0.0938,0.0879, 0.0619, 6.854713)) + 50.98931

# Berkeley parameters
berk.sim <- function(iteration) arima.sim(n=96, list(order=c(1,0,1), ar=c(0.8762), ma=c(-0.6531)), sd=c(0.1032, 0.1612, 6.836614)) + 28.40601 

# San Diego parameters
sd.sim <- function(iteration) arima.sim(n=96, list(order=c(2,0,0), ar=c(0.3605,0.1875), ma=NULL), sd=c(0.1003, 0.1018, 3.203321)) + 30.72144 

# SF paramaters
sf.sim <- function(iteration) arima.sim(n=96, list(order=c(1,0,0), ar=c(0.3151), ma=NULL), sd=c(0.0976,5.014734)) + 46.65183 

# Stockton parameters
stock.sim <- function(iteration) arima.sim(n=96, list(order=c(1,0,0), ar=c(0.3440), ma=NULL), sd=c(0.0978, 7.90195)) + 54.58181

# main function

shock.inner <- function(iteration,m,n,c) {
set.seed(iteration)

library(tsoutliers) 
library(forecast)
library(KFAS)
library(wavethresh)
library(EbayesThresh)

source('./scripts/arima.R')
source("./scripts/tsoutliers.R")
source("./scripts/kfs.R")
source("./scripts/tsay.R")
source("./scripts/swavelet.R")
source("./scripts/hwavelet.R")
source("./scripts/ebt_wavelet.R")
source("./scripts/detectO.R")

  # simulate time series 
  ts1 <- city[[c]](iteration)
  
  # print interation so you can track the simulation progress
  print(iteration)

  # randomly select n points to add shocks
  shocks <- sample(1:length(ts1), n, rep=F)
  
  # add shocks of size m
  ssize <- rep(m,length(shocks))
  
  tso <- ts1
  for (s in 1:length(shocks)) {	
    ts1[shocks[s]] <- ts1[shocks[s]]*(1+ssize[s]) 
  }

  ##########################################################################
                 # Measuring accuracy across methods #
  ##########################################################################
  
  ####### Arima #######
  arima <- ar.out(ts1, shocks)

  ####### Kalman ######
  
  kalman <- kfs.out(ts1, shocks)

  ###### Wavelet ######
  swave <- s.wave.out(ts1, shocks)

  ###### Outlier detection ######
  detectO <- d.out(ts1,shocks)

  out <- cbind(arima,kalman,swave,detectO)
  return(out)
}

# Define city vector
city <- c(stock.sim, la.sim, oak.sim, rich.sim, fres.sim, sac.sim, berk.sim, sd.sim, sf.sim)
names(city) <- c("stock", "la", "oak", "rich", "fres", "sac", "berk", "sd", "sf")

############################## Run program for each city #############################

for (c  in 1:length(city)) {
  
  for  (n in shock.num ){
    for (m in shock.mag) {
    	
    print (paste("city =", names(city)[[c]],"n=",n,"m=",m))

    table <- lapply(1:1000, shock.inner,m=m,n=n,c=c)
   
  results <- na.omit(Reduce("+",table))
  colnames(results) <- c("Arima","Kalman","SoftWavelet","DetectO")

  write.csv(results, file = paste0("filepath",names(city)[[c]],"/results_",names(city)[[c]],"n",n,"m",m,".csv"))
    }
  }
}

##########################################################################
                 # Summarizing results #
##########################################################################

sensitivity <- list()
specificity <- list()

for (s in seq(10,60, by=10)) {
  sensitivity[[(s/10)]] <- data.frame(matrix(ncol=5, nrow=9))
  names(sensitivity[[(s/10)]]) <- c("City","Arima","Kalman","ST Wavelet","Detect AO")
  names(sensitivity)[[(s/10)]] <- paste0("sensitivity",s)
  
}

for (s in seq(10,60, by=10)) {
  specificity[[(s/10)]] <- data.frame(matrix(ncol=5, nrow=9))
  names(specificity[[(s/10)]]) <- c("City","Arima","Kalman","ST Wavelet","Detect AO")
  names(specificity)[[(s/10)]] <- paste0("specificity",s)
  
}

#### Read in csv files produced above and summarize 

for (c in 1:length(cities)) {
  
  city <- cities[c]
  
  df_r <- data.frame(matrix(ncol=6, nrow=50))
  df_a <- data.frame(matrix(ncol=6, nrow=50))
  
  colnames(df_r) <- c("Number","Magnitude","Arima","Kalman","ST Wavelet","Detect AO")
  colnames(df_a) <- c("Number","Magnitude","Arima","Kalman","ST Wavelet","Detect AO")
  
  for(n in 1:10) {
    for (m in 1:5) {
      df <- read.csv(paste0("./results/simulation output/",city,"/results_",city,"n",n,"m0.",m,".csv"))
      df_r[5*(n) + m - 5,1] <-n
      df_r[5*(n) + m - 5,2] <- m*10
      df_a[5*(n) + m - 5,1] <-n
      df_a[5*(n) + m - 5,2] <- m*10 
      for (i in 2:5) {
        df_r[5*(n) + m - 5,i+1] <- df[1,i]/10
        df_a[5*(n) + m - 5,i+1] <- 100*(96-n - df[2,i]/1000)/(96-n)
      }
    }
  }

  for (s in seq(10,60, by=10)) {

     if (s<=50) {
  sensitivity[[s/10]][c,] <- c(city,colMeans(df_r[df_r$Magnitude==s,])[3:6])
  specificity[[s/10]][c,] <- c(city,colMeans(df_a[df_a$Magnitude==s,])[3:6])
    }
    else {
    sensitivity[[s/10]][c,] <- c(city,colMeans(df_r)[3:6])
    specificity[[s/10]][c,] <- c(city,colMeans(df_a)[3:6])
     }
  write.csv(sensitivity[[s/10]],file=paste0("/Users/dana/Documents/Research Projects/Violence Shock Identification/results/tables/sensitivity",s,".csv"))
}
